# Supplementary material for: Complex-Valued 2D Gaussian Representation for Computer-Generated Holography
Source: arXiv:2511.15022 source file (2026-06-25)
Supplement: Supplementary file 1 [file supplementary.tex]

\documentclass[runningheads]{llncs}

% ---------------------------------------------------------------
% Standalone ECCV 2026 Supplementary Material (Electronic Supplementary
% Material / ESM). This compiles INDEPENDENTLY of manuscript.tex so that
% the main camera-ready PDF and the supplementary PDF are separate files,
% as required by the ECCV 2026 / Springer LNCS submission policies.
% ---------------------------------------------------------------

% Camera-ready version
\usepackage[year=2026]{eccv}

% Commonly used abbreviations (\eg, \ie, \etc, \cf, \etal, etc.)
\usepackage{eccvabbrv}

% Import additional packages from preamble (shared with the main paper)
\input{preamble}

% The "axessiblity" package can be found at: https://ctan.org/pkg/axessibility?lang=en
\usepackage[accsupp]{axessibility}

% ---------------------------------------------------------------
% Hyperref package
\usepackage{hyperref}

% Support for ORCID icon
\usepackage{orcidlink}
\usepackage{colortbl}
\definecolor{lightorange}{rgb}{1,0.9,0.7}
\definecolor{lightred}{rgb}{1,0.4,0.4}
\definecolor{lightgreen}{rgb}{0.6,1,0.3}
\definecolor{forestgreen}{rgb}{0.133, 0.545, 0.133}
\definecolor{lightyellow}{rgb}{1,1.0,0.6}

\begin{document}

% Supplementary content (its own title is set inside this file)

% Supplementary content (its own title is set inside this file)

% ---- Bibliography ----
\bibliographystyle{splncs04}
\bibliography{main}

% ---- Bibliography ----
\bibliographystyle{splncs04}
\bibliography{main}

\end{document}
